# Supplementary material for: Negative Differential Resistance in Spin-Crossover Molecular Devices
Source: arXiv:2206.13767 source file (2022-08-10)
Supplement: Supplementary file 1 [file Supporting_information.pdf]

Supporting information for

# Negative Differential Resistance in Spin Crossover Molecular Devices

Dongzhe Li[1,2,*], Yongfeng Tong[3], Kaushik Bairagi[3], Massine Kelai[3], Yannick J. Dappe[4], Jerome Lagoute[3], Yann Girard[3], Sylvie Rousset[3], Vincent Repain[3], Cyrille Barreteau[4], Mads Brandbyge[1,5], Alexander Smogunov[4], and Amandine Bellec[3,*]

[1] Department of Physics, Technical University of Denmark, DK-2800 Kongens Lyngby, Denmark
[2] CEMES, Université de Toulouse, CNRS, 29 rue Jeanne Marvig, F-31055 Toulouse, France
[3] Université Paris Cité, CNRS, Laboratoire Matériaux et Phénomènes Quantiques UMR7162, 75013 Paris, France
[4] SPEC, CEA, CNRS, Université Paris-Saclay, CEA Saclay, Gif-sur-Yvette F-91191, France
[5] Center for Nanostructured Graphene, Technical University of Denmark, DK-2800 Kongens Lyngby, Denmark

*E-mail: dongzhe.li@cemes.fr, amandine.bellec@u-paris.fr

## Section I. Experimental details

The FeMPz molecules have been synthetised as reported in Ref. 1. All the samples have been prepared and measured under ultra-high vacuum in a base pressure of $10^{-10}$ mbar. Before the molecule deposition, the metallic substrates, namely Au(111) on mica or Cu(111) single crystal, were cleaned by Argon sputtering (900 eV for Au and 600 eV for Cu) and annealing (320 °C for Au and 450 °C for Cu) cycles. The HOPG substrate was first cleaved using tap in ambiant conditions, and then annealed up to 120 °C under UHV. The FeMPz molecules were then sublimated on the bare substrates from a crucible at a temperature of around 85 °C to have a sub-monolayer coverage. During the deposition, the substrate was kept at 5 K. After the deposition the samples were annealed at room temperature to enable the formation of molecular islands. For all the substrates reported here the FeMPz molecules self-assembled in dense molecular islands. The measurements were done using a low temperature STM (Scienta-Omicron) operating at 5 K or 78 K.

## Section II. Computational details

The geometry and the electronic properties have been calculated using plane-wave ab initio QUANTUM ESPRESSO[2] package with the PBE exchange-correlation functional. Subsequent spin transport calculations were done using TRANSIESTA[3,4] which employs the non-equilibrium Green's function (NEGF) formalism combined with DFT.

The valence–electron wavefunctions were expanded in a basis set of local orbitals in SIESTA[5,6]. These SIESTA basis parameters, as we have checked, produce accurately the results and trends obtained by QE. The pseudopotentials were taken from Ref. 7 where the parameters have been carefully checked, producing a good agreement with plane-wave ab initio code. The PBE functional, the DZP basis-set, and an energy cutoff for the real-space mesh of 300 Ry were used. We used 6×6 in-plane periodicity in order to avoid artificial interactions between repeating images of molecules due to the periodic boundary conditions. The density matrix and Green's functions were converged self-consistently using 3×3 **k** points, while for transmission calculations, a denser 12×12 **k**-point mesh was employed. Physical quantities like transmission, *I-V* characteristics, and the projected density of states (PDOS) were extracted using TBTRANS, and SISL[8].

## Section III. Spectroscopy of FeMPz molecules on Au(111) at 78 K

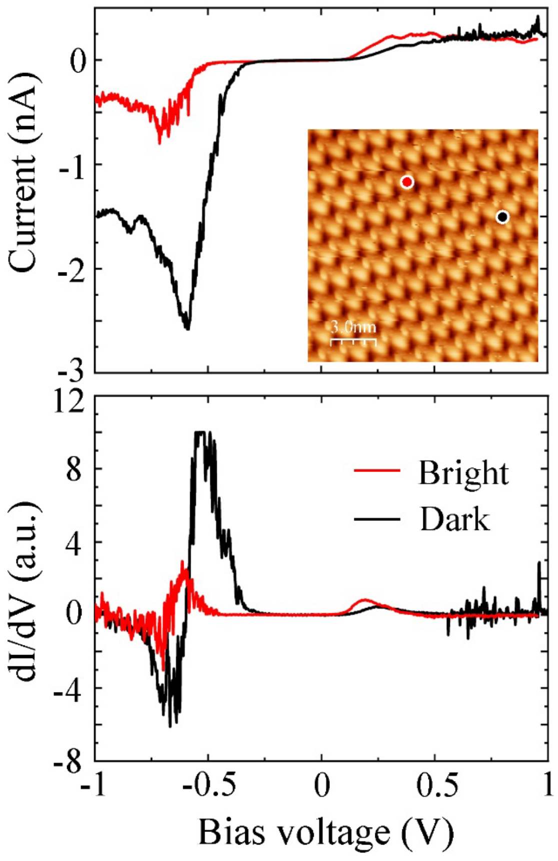


Figure S 1: STS measurements at 78 K on a one-monolayer high island of FeMPz grown on Au(111). Inset, 15×15 nm$^2$ topographic STM image on which the position at which the curves have been acquiered are added (V=0.3 V, I=200 pA).

**Section IV. Spectroscopy of FeMPz molecules on HOPG: switching**

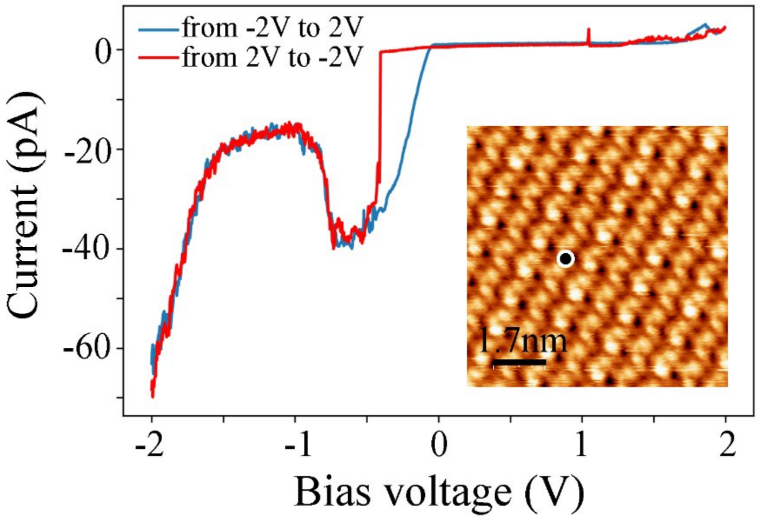


Figure S 2: *I-V* curves acquiered from −2 V to 2 V (blue curve) and from 2 V to −2 V (red curve) on the same molecule in a monolayer on HOPG. Inset, 8.5×8.5 $nm^2$ STM topographic image (V=-1.5 V, I=20 pA).

**Section V. Spectroscopy of FeMPz molecules adsorbed on the tip**

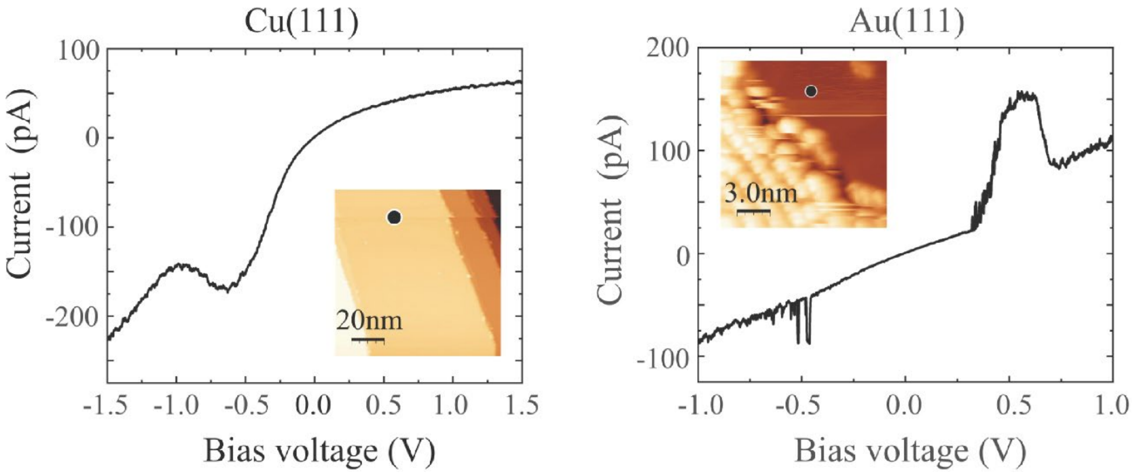


Figure S 3: *I-V* curves acquired just after picking up the molecules. (a) *I-V* curve recorded over Cu(111). Inset, 100×100 $nm^2$ topographic image (-2V, 300pA) with the tip position during the *I-V* curve recording (dot). (b) *I-V* curve recorded over Au(111). Inset, 15×15 $nm^2$ topographic image (0.3V, 20pA) with the tip position during the *I-V* curve recording (dot).

## Section VI. Bias-dependent transmission functions

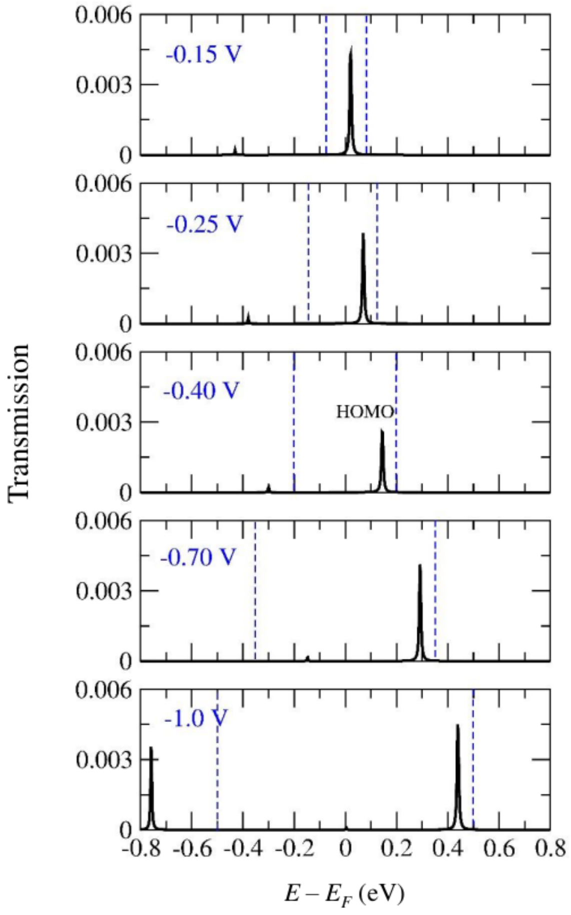


Figure S 4: The transmission coefficients spectra under the bias voltages 0.15, -0.25, -0.40, -0.70, and -1.0 V. The HOMO resonance peak follows the Fermi energy of the surface, and its amplitude changes with respect to the bias voltage. Dotted lines in each panel represent the chemical potential window.

## Section VII. Tip and surface coupling strength projected on HOMO

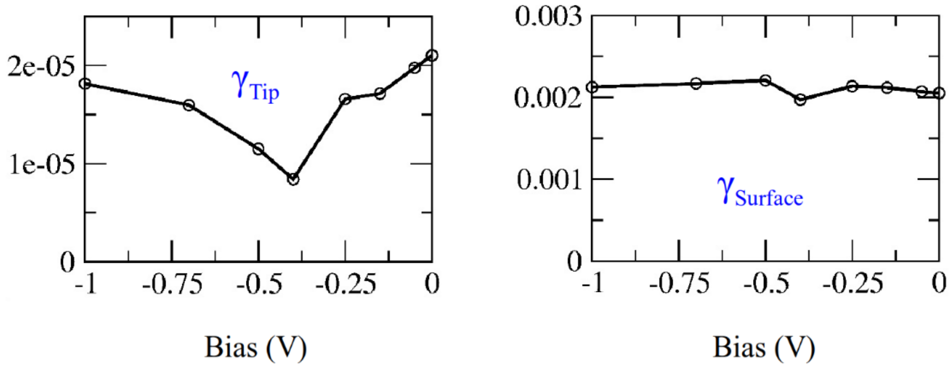


Figure S 5: Calculated $\gamma_{tip}$ (left) and $\gamma_{Surface}$ (right) projected on HOMO. The $\gamma_{tip}$ changes dramatically with respect to the bias voltage while $\gamma_{tip}$ remain almost the same.

## Section VIII. Free standing SCO: DFT+*U*

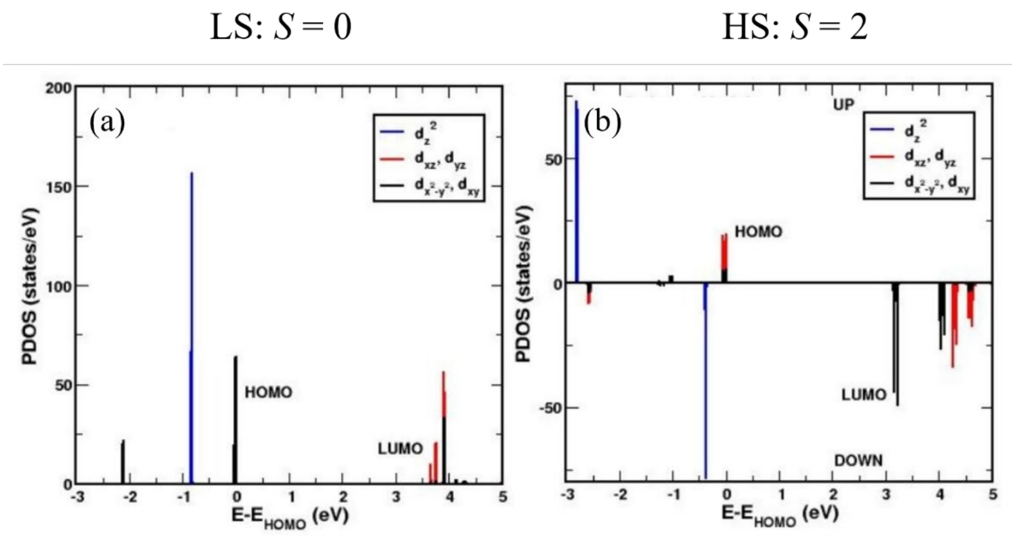


Figure S 6: PDOS of free-standing SCO for LS (a) and HS (b). All the calculations have been done at the DFT+*U* level, with $U = 4$ eV. The HOMO-1 is from localized dz2 orbital for both LS and HS states.

## References


**[1]** O. Iasco, M.-L. Boillot, A. Bellec, R. Guillot, E. Riviere, S. Mazerat, S. Nowak, D. Morineau, A. Brosseau, F. Miserque, et al., J. Mater. Chem. C **5**, 11067 (2017).

**[2]** P. Giannozzi, S. Baroni, N. Bonini, M. Calandra, R. Car, C. Cavazzoni, D. Ceresoli, G. L. Chiarotti, M. Cococcioni, I. Dabo, et al., J. Phys. Condens. Matter **21**, 395502 (2009).

**[3]** M. Brandbyge, J.-L. Mozos, P. Ordejón, J. Taylor, and K. Stokbro, Phys. Rev. B **65**, 165401 (2002).

**[4]** N. Papior, N. Lorente, T. Frederiksen, A. García, and M. Brandbyge, Comput. Phys. Commun. **212**, 8 (2017).

**[5]** J. M. Soler, E. Artacho, J. D. Gale, A. García, J. Junquera, P. Ordejón, and D. Sánchez-Portal, J. Phys. Condens. Matter **14**, 2745 (2002).

**[6]** A. García, N. Papior, A. Akhtar, E. Artacho, V. Blum, E. Bosoni, P. Brandimarte, M. Brandbyge, J. I. Cerdá, F. Corsetti, et al., J. Chem. Phys **152**, 204108 (2020).

**[7]** P. Rivero, V. M. García-Suárez, D. Pereñiguez, K. Utt, Y. Yang, L. Bellaiche, K. Park, J. Ferrer, and S. Barraza-Lopez, Comput. Mater. Sci **98**, 372 (2015).

**[8]** N. Papior, sisl: v0.11.0 (2021), URL https://doi.org/10.5281/zenodo.597181.
